# Supplementary material for: Heterogeneous Wasserstein Discrepancy for Incomparable Distributions
Source: arXiv:2106.02542 source file (2021-10-12)
Supplement: Supplementary file 1 [file supplement.tex]

\documentclass{article} % For LaTeX2e
\usepackage{iclr2022_conference,times}

% Optional math commands from https://github.com/goodfeli/dlbook_notation.
% \input{math_commands.tex}

%%%%%%%%%%%%%%%%%%%%%%%%%%%%%%%%%%%%%%%%%%%%%%%%%%%%%%%%%%%%%%

\usepackage[utf8]{inputenc} % allow utf-8 input
\usepackage[T1]{fontenc}    % use 8-bit T1 fonts
\usepackage{hyperref}       % hyperlinks
\usepackage{url}            % simple URL typesetting
\usepackage{booktabs}       % professional-quality tables
\usepackage{amsfonts}       % blackboard math symbols
\usepackage{nicefrac}       % compact symbols for 1/2, etc.
\usepackage{microtype}      % microtypography
\usepackage{xcolor}         % colors
\usepackage{algorithm}
\usepackage{algpseudocode}
\usepackage{wrapfig}
%\usepackage{subcaption}

% Recommended, but optional, packages for figures and better typesetting:
%\usepackage{chngcntr}
%\counterwithin{figure}{section} 
\usepackage{graphicx}
\usepackage{subfigure}
\usepackage{booktabs} % for professional tables
\usepackage{macros} % Macros

%%%%%%%%%%%%%%%%%
% LINK APPENDIX %
%%%%%%%%%%%%%%%%%
\usepackage{xcite}
\usepackage{xr}
\makeatletter
\newcommand*{\addFileDependency}[1]{% argument=file name and extension
  \typeout{(#1)}
  \@addtofilelist{#1}
  \IfFileExists{#1}{}{\typeout{No file #1.}}
}
\makeatother

\externaldocument{main}

%%%%%%%%%%%%
% COMMENTS %
%%%%%%%%%%%%
\usepackage[textwidth=2.0cm, textsize=tiny]{todonotes} % for writting

\definecolor{bnfj}{rgb}{0.600000,0.200000,1.000000}

%%%%%%%%
% TIKZ %
%%%%%%%%%
\usepackage{tikz}
\usetikzlibrary{matrix}
\usepackage{pgfplots}
\usepgfplotslibrary{patchplots}
\usetikzlibrary{patterns, positioning, arrows}

%%%%%%%%%%%%%%%%%%%%%%%%%%%%%%%%%%%%%%%%%%%%%%%%%%%%%%%%%%%

%%% TITLE
\title{Supplemental Material to ``Heterogeneous Wasserstein Discrepancy for Incomparable Distributions''}

% The \author macro works with any number of authors. There are two commands
% used to separate the names and addresses of multiple authors: \And and \AND.
%
% Using \And between authors leaves it to LaTeX to determine where to break the
% lines. Using \AND forces a line break at that point. So, if LaTeX puts 3 of 4
% authors names on the first line, and the last on the second line, try using
% \AND instead of \And before the third author name.

\author{%
  David S.~Hippocampus\thanks{Use footnote for providing further information
    about author (webpage, alternative address)---\emph{not} for acknowledging
    funding agencies.} \\
  Department of Computer Science\\
  Cranberry-Lemon University\\
  Pittsburgh, PA 15213 \\
  \texttt{hippo@cs.cranberry-lemon.edu} \\
  % examples of more authors
  % \And
  % Coauthor \\
  % Affiliation \\
  % Address \\
  % \texttt{email} \\
  % \AND
  % Coauthor \\
  % Affiliation \\
  % Address \\
  % \texttt{email} \\
  % \And
  % Coauthor \\
  % Affiliation \\
  % Address \\
  % \texttt{email} \\
  % \And
  % Coauthor \\
  % Affiliation \\
  % Address \\
  % \texttt{email} \\
}

\begin{document}

\maketitle

\appendix 

\input{appendix}

% \FloatBarrier
\bibliography{biblio}
\bibliographystyle{iclr2022_conference}

%%%%%%%%%%%%%%%%%%%%%%%%%%%%%%%%%%%%%%%%%%%%%%%%%%%%%%%%%%%%

\end{document}
